# Supplementary material for: Pricing Social Visibility Service in Online Social Networks: Modeling and Algorithms
Source: arXiv:2106.10473 source file (2021-06-19)
Supplement: Supplementary file 1 [file appendix.tex]

% !TEX root = supplementary.tex

\section{\bf Proof to Lemmas and Theorems}  
\noindent
\textbf{Proof of Theorem \ref{thm:hard:prob2}.}
Given an instance of set cover problem,
as shown in Fig.~\ref{fig:nphard_prob} 
we can construct an instance of Problem~\ref{prob:sub-problem1} as follows:
$\tau = 2, p=1, \alpha = 0, 
\widetilde{R}(p) = \{r\},
\widetilde{S}(p) =\{s_1,...,s_{|\widetilde{S}(p)|}\}, 
\mathcal{U}=\widetilde{R}(p)\cup \widetilde{S}(p)\cup X$ . 
Each element $e \in  {N}$ in set cover problem 
will corresponds to a node $u \neq r$ in the network.
And each subset $T_i$ will corresponds to nodes in the set $\mathcal{V}(s_i,1;\mathcal{G}) $, e.g., $T_1$ corresponds to $\mathcal{V}(s_1,1;\mathcal{G}) = \{s_1, x_1,x_2,x_3\}$.
Then according to our previous derivation,
the total visibility increase of $\widetilde{R}(p)$ after selecting 
$\mathcal{M} = \{s_i| i\in \mathcal{I} \subseteq [m], |\mathcal{I}|\leq b\}$ 
where $ m =  \lvert \widetilde{S}(p)  \rvert$,  
is
\begin{align}
&I(p,\mathcal{M})  \notag \\
= &\sum_{u\in \widetilde{R}(p)} I_u(p,\mathcal{M})  \notag  \\
%= & f_1(\mathcal{M} \times \mathcal{R}) \\
= & \sum_{u \in  \widetilde{R}(p)} \lvert
	\medcup_{l \in \mathcal{M} \times  \widetilde{R}(p)} \mathcal{V}(l^s,\tau - 1 - D(l^e , r;\mathcal{G});\mathcal{G}) 
	\setminus \mathcal{V}(r, \tau;\mathcal{G})  \rvert   \notag\\
	%F(\mathcal{\mathcal{L}}) &=\sum_{r \in \mathcal{R}} \lvert \medcup_{l \in \mathcal{\mathcal{L}}} \mathcal{V}(l^s,\tau - 1 - d(l^e \to r)) \setminus \mathcal{V}(r, \tau) \rvert \\
= &\lvert \cup_{i \in \mathcal{I}}  \mathcal{V}(s_i,1;\mathcal{G})  \rvert   \label{eq:setcover},  
\end{align}
where $l^s$ and $l^e$ are the start node and the end node 
of  each link  $l\in  \mathcal{M} \times \widetilde{R}(p)$
and Equation~\eqref{eq:setcover} is corresponding to the result of set cover problem. 
It is obvious that there is a subset of size $b$ that satisfies $R(p,q,\mathcal{M})\geq k$ 
for $p=1, \alpha=0$
if and only if there is a subset of size $b$ in the set cover instance that cover at least $k$ elements.
\done

\begin{figure}[H] %H为当前位置，!htb为忽略美学标准，htbp为浮动图形
	\centering %图片居中
	\includegraphics[width=0.24\textwidth]{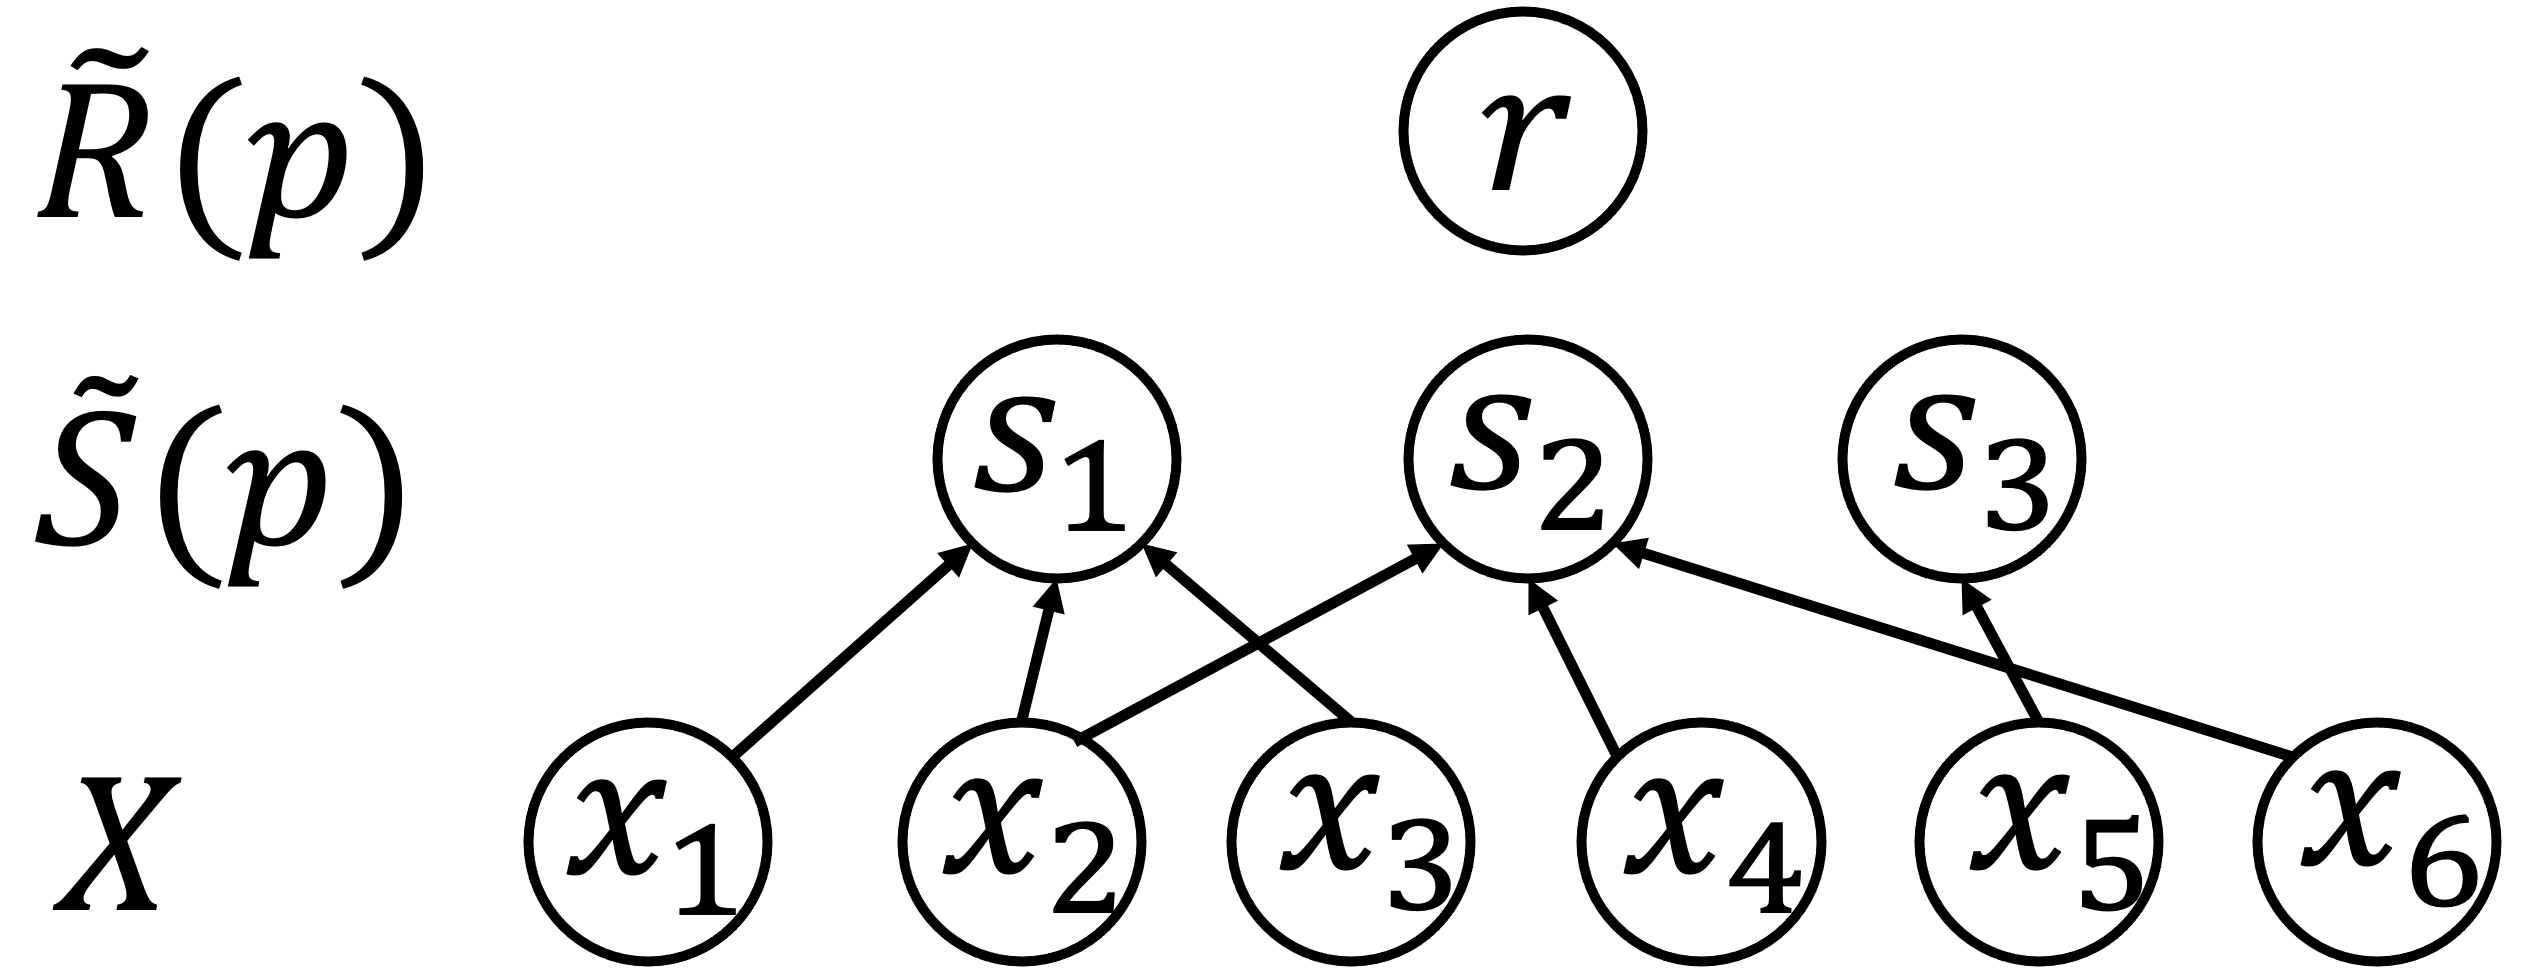} %插入图片，[]中设置图片大小，{}中是图片文件名
	\caption{Network of our problem.} %最终文档中希望显示的图片标题
	\label{fig:nphard_prob} %用于文内引用的标签
\end{figure}

\noindent
\textbf{Proof of Theorem \ref{thm:submodular}.}
We first prove $R(p,q, \mathcal{M})$ is monotone increasing and submodular with $\mathcal{M}$.
Let	$l = (l^s,\l^e)$ be a directed link in set of new added links $\mathcal{M} \times \widetilde{R}(p)$, 
where $l^s$ is the start node (supplier) and 
$l^e$ is the end node (requester) of link $l$.
The total visibility increase of requesters $\widetilde{R}(p)$
after adding new links $\mathcal{M} \times \widetilde{R}(p)$ is 
\begin{align}
	\label{eq:close}
	&I(p,\mathcal{M})\\ \notag
	=& \sum_{r\in \widetilde{R}(p) } \big| 
	\medcup_{l \in \mathcal{M} \times \widetilde{R}(p) } \mathcal{V}(l^s,\tau - 1 - D(l^e, r; \mathcal{G}); \mathcal{G}) 
	\setminus \mathcal{V}(r, \tau;\mathcal{G}) \big|.
\end{align}
\noindent
According to Equation~\eqref{eq:close}, 
for $\forall \mathcal{M}_1 \subseteq \mathcal{M}_2$, obviously we have $R(p,q, \mathcal{M}_1) \leq R(p,q, \mathcal{M}_2)$.
\begin{align}
	& I(p, \mathcal{M}\cup \{ \bar{u} \}) 
	- I(p, \mathcal{M} ) \\ \notag
	=& \sum_{r\in \widetilde{R}(p) } \big| \medcup_{l \in (\mathcal{M}\cup \{ \bar{u} \} )\times \widetilde{R}(p)} \mathcal{V}(l^s,\tau - 1 - D(l^e , r; \mathcal{G});\mathcal{G}) \setminus \mathcal{V}(r, \tau;\mathcal{G}) \big| \\ \notag
	& - \sum_{r\in \widetilde{R}(p)} \big| \medcup_{l \in \mathcal{M} \times \widetilde{R}(p) } \mathcal{V}(l^s,\tau - 1 - D(l^e , r;\mathcal{G});\mathcal{G}) \setminus \mathcal{V}(r, \tau;\mathcal{G})\big| \\ \notag
	=& \sum_{r\in \widetilde{R}(p)} \big|[\medcup_{l \in (\mathcal{M}\cup \{ \bar{u} \} )\times \widetilde{R}(p) } \mathcal{V}(l^s,\tau - 1 - D(l^e , r; \mathcal{G});\mathcal{G}) \setminus \mathcal{V}(r, \tau;\mathcal{G})] \\ \notag
	&\setminus [\medcup_{l \in \mathcal{M} \times \widetilde{R}(p)} \mathcal{V}(l^s,\tau - 1 - D(l^e, r; \mathcal{G});\mathcal{G}) \setminus \mathcal{V}(r, \tau;\mathcal{G})]\big| \\ \notag
	= & \sum_{r\in \widetilde{R}(p)} \big| \medcup_{l \in \{\bar{u}\}\times \widetilde{R}(p)} \mathcal{V}(\bar{l}^s,\tau - 1 - D(\bar{l}^e , r; \mathcal{G});\mathcal{G}) \setminus \mathcal{V}(r, \tau;\mathcal{G}) \\ \notag 
	&\setminus \medcup_{l \in \mathcal{M} \times \widetilde{R}(p)} \mathcal{V}(l^s,\tau - 1 - D(l^e , r; \mathcal{G});\mathcal{G}) \big|
\end{align}
For $\forall \mathcal{M}_1 \subseteq \mathcal{M}_2$, for $\forall r \in \widetilde{R}(p)$
we have 
\begin{align}
	\medcup_{l \in \mathcal{M}_1 \times \widetilde{R}(p) }  & \mathcal{V}(l^s,\tau - 1 - D(l^e, r;\mathcal{G});\mathcal{G}) \\ \notag
	& \subseteq  \medcup_{l \in \mathcal{M}_2 \times \widetilde{R}(p)}  \mathcal{V}(l^s,\tau - 1 - D(l^e, r;\mathcal{G});\mathcal{G}),
\end{align}
and
\begin{align}
I(p, \mathcal{M}_1\cup \{ \bar{u} \}) - I(p, \mathcal{M}_1 ) \geq I(p, \mathcal{M}_2 \cup \{ \bar{u} \}) - I(p, \mathcal{M}_2 ).
%	f(\mathcal{M}_1\cup\{ \bar{u} \} \times \mathcal{R} ) & - f(\mathcal{M}_1 \times \mathcal{R} )  \\ \notag
%	& \geq f(\mathcal{M}_2\cup\{ \bar{u}\} \times \mathcal{R}) - f(\mathcal{M}_2 \times \mathcal{R}).
\end{align}
which indicates $I(p,\mathcal{M})$ is submodular with $\mathcal{M}$.
Thus, we prove $I(p,\mathcal{M})$ is monotone and submodular with $\mathcal{M}$.
Since the objective function is linear to total increase of participating requesters, i.e., $R(p,q, \mathcal{M}) =(p-q)I(p,\mathcal{M})$, the objective function is also monotone and submodular with $\mathcal{M}$.
\done

\noindent
%\textbf{Remark:} Theorem~\ref{thm:greedy_ratio} states that 
%our solution can achieve a high theoretical guarantee .
\textbf{Proof of Theorem \ref{thm:greedy_ratio}.} 
Let $\hat{\mathcal{M}}^\ast_{i}$ be the supplier selected in $i$-th round in Algorithm~\ref{alg:greedy} and $\mathcal{M}^\ast$ denote the optimal set of suppliers via exhaustive search.
We have proved $R(p,q, \mathcal{M})$ is monotone and submodular with $\mathcal{M}$, so we have
% TODO 证明推论1 https://zhuanlan.zhihu.com/p/52512602
\begin{align*}
	& R(p,q, \mathcal{M}^\ast) \\
	\leq & R(p,q, \hat{\mathcal{M}}^\ast_{i-1}) + \\
	&\sum_{u \in \mathcal{M}^\ast \setminus  \hat{\mathcal{M}}^\ast_{i-1} } 
	[	R(p,q, \hat{\mathcal{M}}^\ast_{i-1} \cup \{u\} ) - 	R(p,q, \hat{\mathcal{M}}^\ast_{i-1} )] \\
	\leq &
	R(p,q, \hat{\mathcal{M}}^\ast_{i-1}) + 
	\sum_{u \in \mathcal{M}^\ast \setminus  \hat{\mathcal{M}}^\ast_{i-1} } 
	[R(p,q, \hat{\mathcal{M}}^\ast_{i} ) - 	R(p,q, \hat{\mathcal{M}}^\ast_{i-1} )] \\	    
	\leq &
		R(p,q, \hat{\mathcal{M}}^\ast_{i-1}) + 
	b [R(p,q, \hat{\mathcal{M}}^\ast_{i} ) - 	R(p,q, \hat{\mathcal{M}}^\ast_{i-1} )] 
\end{align*}
Minus $b 	R(p,q, \mathcal{M}^\ast) $ both sides, we have
\begin{align*}
	&R(p,q, \mathcal{M}^\ast)  - b R(p,q, \mathcal{M}^\ast) \\
	 \leq & R(p,q, \hat{\mathcal{M}}^\ast_{i-1}) + b R(p,q, \hat{\mathcal{M}}^\ast_{i} ) - b R(p,q, \hat{\mathcal{M}}^\ast_{i-1} ) -b R(p,q, \mathcal{M}^\ast) 
	%\frac{b-1}{b} [f(S_{i-1}) - f(S^\ast)]&\leq  f( \hat{\mathcal{L}}^\ast_{i-1}) - f( \mathcal{L}^\ast)
\end{align*}
Rewrite it we can get
\begin{align*}
	&R(p,q,\hat{\mathcal{M}}^\ast_{i}) - R(p,q,\mathcal{M}^\ast)  \\
	\geq &\frac{b-1}{b} [R(p,q, \hat{\mathcal{M}}^\ast_{i-1}) - R(p,q, \mathcal{M}^\ast) ] \\
	\geq &(\frac{b-1}{b})^2 [R(p,q, \hat{\mathcal{M}}^\ast_{i-2}) - R(p,q, \mathcal{M}^\ast) ] \\
	&\cdots\\
	\geq &(\frac{b-1}{b})^b [R(p,q,\emptyset) - R(p,q, \mathcal{M}^\ast) ] \\ 
\end{align*}
Note that 
\begin{align*}
	(\frac{b-1}{b})^b  \leq 1/e
\end{align*}
Thus, we have
\begin{align*}
	 &R(p,q, \hat{\mathcal{M}}^\ast_{i})  \\
	 \geq & (\frac{b-1}{b})^b [ R(p,q,\emptyset) -  R(p,q,\mathcal{M}^\ast) ] +   R(p,q, \mathcal{M}^\ast)   \\ 
	 \geq  & (1-1/e)  R(p,q, \mathcal{M}^\ast) 
\end{align*}
Thus, we complete the prove of approximation ratio.
\done

\noindent
\textbf{Analysis of the condition of potential participating users.}
Let $\hat{\mathcal{M}}^\ast (p_{\text{DS}}^\ast, q_{\text{DS}}^\ast)$ %# $\mathcal{M}^\ast$ 
 be the optimal set of participating suppliers 
and $\hat{\mathcal{M}}^\ast (p_{\text{DS}}^\ast, q_{\text{DS}}^\ast) = b$.
We define a cooperative game, where
the coalition is the supplier set $\hat{\mathcal{M}}^\ast (p_{\text{DS}}^\ast, q_{\text{DS}}^\ast)$, 
each supplier $u \in \hat{\mathcal{M}}^\ast (p_{\text{DS}}^\ast, q_{\text{DS}}^\ast)$ 
can be regarded as an individual player,
and characteristic function of set $\mathcal{M} \subseteq \hat{\mathcal{M}}^\ast (p_{\text{DS}}^\ast, q_{\text{DS}}^\ast)$ of players in the cooperation game 
is %\nu( \mathcal{M})
$I(p_{\text{DS}}^\ast, \mathcal{M}) $.
%The Shapley value of each individual supplier $u \in  \hat{\mathcal{M}}^\ast$ can be computed as follows: 
We use the Shapley value to divide $I(p_{\text{DS}}^\ast, \hat{\mathcal{M}}^\ast (p_{\text{DS}}^\ast, q_{\text{DS}}^\ast))$.
Formally, each participating supplier $u \in \hat{\mathcal{M}}^\ast (p_{\text{DS}}^\ast, q_{\text{DS}}^\ast)$ 
has the following share of contribution to the total visibility increase
%$\phi_u (p_{\text{DS}}^\ast, 
%\hat{\mathcal{M}}^\ast (p_{\text{DS}}^\ast, q_{\text{DS}}^\ast))$
%computed as Equation~\eqref{eq:shap}. 
\begin{align*}
& 
\phi_u (p_{\text{DS}}^\ast, 
\hat{\mathcal{M}}^\ast (p_{\text{DS}}^\ast, q_{\text{DS}}^\ast)) 
\\
& 
= 
\sum_{\mathcal{M}\subseteq {
		\hat{\mathcal{M}}^\ast (p_{\text{DS}}^\ast, q_{\text{DS}}^\ast)
	} \setminus\{u\}  }  
\frac{|\mathcal{M}|!
	(|\hat{\mathcal{M}}^\ast (p_{\text{DS}}^\ast, q_{\text{DS}}^\ast)| 
	-|\mathcal{M}|-1)!}{|\hat{\mathcal{M}}^\ast (p_{\text{DS}}^\ast, q_{\text{DS}}^\ast))|!} 
\\
& 
\hspace{0.18in}
\times 
(  
I(p_{\text{DS}}^\ast, 
\mathcal{M}\cup \{u\})
- 
I(p_{\text{DS}}^\ast, 
\mathcal{M}) 
).  
\end{align*}  
Thus, the share of total reward of supplier $u$ is $ \alpha p_{\text{DS}}^\ast  \phi_u (p_{\text{DS}}^\ast, \hat{\mathcal{M}}^\ast (p_{\text{DS}}^\ast, q_{\text{DS}}^\ast)) $.
%\begin{align}
%\label{eq:shapley}
%\phi_u (p, \mathcal{M}^\ast) 
%= \sum_{\mathcal{S}\subset {\mathcal{M}} \setminus\{u\}  }  
%\frac{|\mathcal{S}|!(b-|\mathcal{S}|-1)!}{b!} (  \nu( \mathcal{S}\cup \{u\})  - \nu(\mathcal{S}) ). 
%\end{align}
We define the cost of each participating supplier
 $u \in \hat{\mathcal{M}}^\ast (p_{\text{DS}}^\ast, q_{\text{DS}}^\ast) $ 
is % $q_u \nu(\{u\})$
$q_u I(p_{\text{DS}}^\ast, \{u\}) $, 
%\[
%c_u(p, \mathcal{M}^\ast) = \nu(\{u\}) = q_u I(p, \mathcal{M}^\ast) . 
%\] 
and assume suppliers are risk preferred.
Then, we have the following theorem about the potential of a supplier $u \in \mathcal{S}$  
to participate in the  social visibility boosting service.
\begin{thm}
	Given prices $(p, \alpha p)$, if a supplier $u \in \mathcal{S}$ satisfies $q_u > \alpha p $, 
	then $u$ is not a potential participating supplier, i.e., $u \notin \widetilde{R}(p)$, 
	otherwise, $u \in \widetilde{R}(p)$.
\end{thm}
\noindent
\textbf{Proof.}
The characteristic function is submodular thus subadditive, i.e., 
\[
I(p_{\text{DS}}^\ast, \mathcal{M}_1 \sqcup \mathcal{M}_2)  \leq 
I(p_{\text{DS}}^\ast, \mathcal{M}_1) + I(p_{\text{DS}}^\ast,  \mathcal{M}_2)
%\nu( \mathcal{M}_1 \sqcup \mathcal{M}_2) \leq \nu(\mathcal{M}_1) + \nu(\mathcal{M}_2).
\] 
According to the \textit{stand-alone test} property of Shapley value, we have
% TODO 加这个property的ref
%$$\phi_l \leq \alpha p  f(\{l\}). $$
\[
\phi_u (p_{\text{DS}}^\ast, \hat{\mathcal{M}}^\ast (p_{\text{DS}}^\ast, q_{\text{DS}}^\ast))  
\leq   I(p_{\text{DS}}^\ast,  \{u\} ) . 
\]
Since $q_u > \alpha p_{\text{DS}}^\ast $, we have
\[
 \alpha p_{\text{DS}}^\ast I( p_{\text{DS}}^\ast , \{u\})  < q_u I( p_{\text{DS}}^\ast, \{u\}). 
\] 
Thus, we have have
\[ 
\alpha p_{\text{DS}}^\ast \phi_u (  p_{\text{DS}}^\ast, \hat{\mathcal{M}}^\ast (p_{\text{DS}}^\ast, q_{\text{DS}}^\ast)) 
<  q_u I( p_{\text{DS}}^\ast, \{u\}),
\]  
which shows that, 
for user $u \in \mathcal{S}$ with $q_u > \alpha p$, 
the reward received of participating supplier $u$ (LHS) can not be greater than the cost of $u$ (RHS),
thus $u$ can not be to participant in the social visibility boosting service. 
Otherwise, if $q_u \leq \alpha$, then $u$ is a potential participating supplier, i.e., $u \in \widetilde{S}(p) $.
\done
