# Supplementary material for: Pricing Social Visibility Service in Online Social Networks: Modeling and Algorithms
Source: arXiv:2106.10473 source file (2021-06-19)
Supplement: Supplementary file 3 [file supplementarySocialVisPricing.pdf]

# Social Visibility Pricing in OSNs: Modeling and Algorithms

Shiyuan Zheng

Dept. of Computer Science & Engineering  
The Chinese University of Hong Kong  
syzheng@cse.cuhk.edu.hk

Hong Xie

College of Computer Science  
Chongqing University  
xiehong2018@cqu.edu.cn

John C.S. Lui

Dept. of Computer Science & Engineering  
The Chinese University of Hong Kong  
cslui@cse.cuhk.edu.hk

**Abstract**—This abstract contains technical proofs to all theorems and lemmas in the main paper.

## I. Proof to Lemmas and Theorems

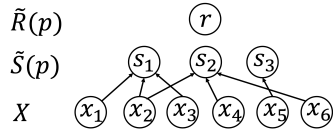

Fig. 1. Network of our problem.

**Proof of Theorem 1.** Given an instance of set cover problem, as shown in Fig. 1 we can construct an instance of Problem 3 as follows:  $\tau = 2$ ,  $\tilde{R}(p) = \{r\}$ ,  $\tilde{S}(p) = \{s_1, \dots, s_{\tilde{S}(p)}\}$ ,  $\mathcal{U} = \tilde{R}(p) \cup \tilde{S}(p) \cup X$ . Each element  $e \in N$  in set cover problem will corresponds to a node  $u \neq r$  in the network. And each subset  $T_i$  will corresponds to nodes in the set  $\mathcal{V}(s_i, 1; \mathcal{G})$ , e.g.,  $T_1$  corresponds to  $\mathcal{V}(s_1, 1; \mathcal{G}) = \{s_1, x_1, x_2, x_3\}$ . Then according to our previous derivation, the total visibility increase of  $\tilde{R}(p)$  after selecting  $\mathcal{M} = \{s_i | i \in \mathcal{I} \subseteq [m], |\mathcal{I}| \leq b\}$  where  $m = |\tilde{S}|$ , is

$$I(p, \mathcal{M}) \quad (1)$$

$$= \sum_{u \in \tilde{R}(p)} I_u(p, \mathcal{M}) \quad (2)$$

$$= \sum_{u \in \tilde{R}(p)} |\cup_{l \in \mathcal{M} \times \tilde{R}(p)} \mathcal{V}(l^s, \tau - 1 - d(l^e, r); \mathcal{G}) \setminus \mathcal{V}(r, \tau; \mathcal{G})|$$

$$= |\cup_{i \in \mathcal{I}} \mathcal{V}(s_i, 1; \mathcal{G})| \quad \text{in this setting}$$

It is obvious that there is a subset of size  $b$  that satisfies  $R(p, q, \mathcal{M}) \geq k$  if and only if there is a subset of size  $b$  in the set cover instance that cover at least  $k$  elements. ■

**Proof of Theorem 2.** We first prove  $R(p, q, \mathcal{M})$  is monotone increasing and submodular with  $\mathcal{M}$ . Let  $l = (l^s \rightarrow l^e)$  be a directed link in set of new added links  $\mathcal{M} \times \tilde{R}(p)$ , where  $l^s$  is the start node (supplier) and  $l^e$  is the end node (requester)

of link  $l$ . The total visibility increase of requesters  $\tilde{R}(p)$  after adding new links  $\mathcal{M} \times \tilde{R}(p)$  is

$$I(p, \mathcal{M}) \quad (4)$$

$$= \sum_{r \in \tilde{R}(p)} |\cup_{l \in \mathcal{M} \times \tilde{R}(p)} \mathcal{V}(l^s, \tau - 1 - d(l^e, r); \mathcal{G}) \setminus \mathcal{V}(r, \tau; \mathcal{G})|.$$

According to Eq. (4), for  $\forall \mathcal{M}_1 \subseteq \mathcal{M}_2$ , obviously we have  $R(p, q, \mathcal{M}_1) \leq R(p, q, \mathcal{M}_2)$ .

$$I(p, \mathcal{M} \cup \{\bar{u}\}) - I(p, \mathcal{M}) \quad (5)$$

$$\begin{aligned} &= \sum_{r \in \tilde{R}(p)} |\cup_{l \in (\mathcal{M} \cup \{\bar{u}\}) \times \tilde{R}(p)} \mathcal{V}(l^s, \tau - 1 - d(l^e, r); \mathcal{G}) \setminus \mathcal{V}(r, \tau; \mathcal{G})| \\ &\quad - \sum_{r \in \tilde{R}(p)} |\cup_{l \in \mathcal{M} \times \tilde{R}(p)} \mathcal{V}(l^s, \tau - 1 - d(l^e, r); \mathcal{G}) \setminus \mathcal{V}(r, \tau; \mathcal{G})| \\ &= \sum_{r \in \tilde{R}(p)} |[\cup_{l \in (\mathcal{M} \cup \{\bar{u}\}) \times \tilde{R}(p)} \mathcal{V}(l^s, \tau - 1 - d(l^e, r); \mathcal{G}) \setminus \mathcal{V}(r, \tau; \mathcal{G})] \\ &\quad \setminus [\cup_{l \in \mathcal{M} \times \tilde{R}(p)} \mathcal{V}(l^s, \tau - 1 - d(l^e, r); \mathcal{G}) \setminus \mathcal{V}(r, \tau; \mathcal{G})]| \\ &= \sum_{r \in \tilde{R}(p)} |\cup_{l \in \{\bar{u}\} \times \tilde{R}(p)} \mathcal{V}(\bar{l}^s, \tau - 1 - d(\bar{l}^e, r); \mathcal{G}) \setminus \mathcal{V}(r, \tau; \mathcal{G}) \\ &\quad \setminus \cup_{l \in \mathcal{M} \times \tilde{R}(p)} \mathcal{V}(l^s, \tau - 1 - d(l^e, r); \mathcal{G})| \end{aligned}$$

For  $\forall \mathcal{M}_1 \subseteq \mathcal{M}_2$ , for  $\forall r \in \tilde{R}(p)$  we have

$$\cup_{l \in \mathcal{M}_1 \times \tilde{R}(p)} \mathcal{V}(l^s, \tau - 1 - d(l^e, r); \mathcal{G}) \quad (6)$$

$$\subseteq \cup_{l \in \mathcal{M}_2 \times \tilde{R}(p)} \mathcal{V}(l^s, \tau - 1 - d(l^e, r); \mathcal{G}),$$

and

$$I(p, \mathcal{M}_1 \cup \{\bar{u}\}) - I(p, \mathcal{M}_1) \geq I(p, \mathcal{M}_2 \cup \{\bar{u}\}) - I(p, \mathcal{M}_2). \quad (7)$$

which indicates  $I(p, \mathcal{M})$  is submodular with  $\mathcal{M}$ . Thus, we prove  $I(p, \mathcal{M})$  is monotone and submodular with  $\mathcal{M}$ . Since the objective function is linear to total increase of participating requesters, i.e.,  $R(p, q, \mathcal{M}) = (p - q)I(p, \mathcal{M})$ , the objective function is also monotone and submodular with  $\mathcal{M}$ . ■

**Proof of Theorem 3.** Let  $\hat{\mathcal{M}}_i^*$  be the supplier selected in  $i$ -th round in Algorithm 1 and  $\mathcal{M}^*$  denote the optimal set of

suppliers via exhaustive search. We have proved  $R(p, q, \mathcal{M})$  is monotone and submodular with  $\mathcal{M}$ , so we have

$$\begin{aligned}
& R(p, q, \mathcal{M}^*) \\
& \leq R(p, q, \hat{\mathcal{M}}_{i-1}^*) + \\
& \quad \sum_{u \in \mathcal{M}^* \setminus \hat{\mathcal{M}}_{i-1}^*} [R(p, q, \hat{\mathcal{M}}_{i-1}^* \cup \{u\}) - R(p, q, \hat{\mathcal{M}}_{i-1}^*)] \\
& \leq R(p, q, \hat{\mathcal{M}}_{i-1}^*) + \sum_{u \in \mathcal{M}^* \setminus \hat{\mathcal{M}}_{i-1}^*} [R(p, q, \hat{\mathcal{M}}_i^*) - R(p, q, \hat{\mathcal{M}}_{i-1}^*)] \\
& \leq R(p, q, \hat{\mathcal{M}}_{i-1}^*) + b[R(p, q, \hat{\mathcal{M}}_i^*) - R(p, q, \hat{\mathcal{M}}_{i-1}^*)]
\end{aligned}$$

Minus  $bR(p, q, \mathcal{M}^*)$  both sides, we have

$$\begin{aligned}
& R(p, q, \mathcal{M}^*) - bR(p, q, \mathcal{M}^*) \\
& \leq R(p, q, \hat{\mathcal{M}}_{i-1}^*) + bR(p, q, \hat{\mathcal{M}}_i^*) - bR(p, q, \hat{\mathcal{M}}_{i-1}^*) - bR(p, q, \mathcal{M}^*)
\end{aligned}$$

Rewrite it we can get

$$\begin{aligned}
& R(p, q, \hat{\mathcal{M}}_i^*) - R(p, q, \mathcal{M}^*) \\
& \geq \frac{b-1}{b} [R(p, q, \hat{\mathcal{M}}_{i-1}^*) - R(p, q, \mathcal{M}^*)] \\
& \geq \left(\frac{b-1}{b}\right)^2 [R(p, q, \hat{\mathcal{M}}_{i-2}^*) - R(p, q, \mathcal{M}^*)] \\
& \quad \dots \\
& \geq \left(\frac{b-1}{b}\right)^b [R(p, q, \emptyset) - R(p, q, \mathcal{M}^*)]
\end{aligned}$$

Note that

$$\left(\frac{b-1}{b}\right)^b \leq 1/e$$

Thus, we have

$$\begin{aligned}
& R(p, q, \hat{\mathcal{M}}_i^*) \\
& \geq \left(\frac{b-1}{b}\right)^b [R(p, q, \emptyset) - R(p, q, \mathcal{M}^*)] + R(p, q, \mathcal{M}^*) \\
& \geq (1 - 1/e) R(p, q, \mathcal{M}^*)
\end{aligned}$$

Thus, we complete the prove of approximation ratio. ■
